# Supplementary material for: Unusual destruction and enhancement of superfluidity of atomic Fermi gases by population imbalance in a one-dimensional optical lattice
Source: arXiv:1904.09576 ancillary file (2020-03-03)
Supplement: Supplementary file 1 [file SI.pdf]

# Supplementary Information
# Unusual destruction and enhancement of superfluidity of atomic Fermi gases by population imbalance in a one-dimensional optical lattice

Qijin Chen,[1,2,3,*] Jibiao Wang,[4,†] Lin Sun,[2] and Yi Yu[5]

[1]*Shanghai Branch, National Laboratory for Physical Sciences at Microscale and Department of Modern Physics, University of Science and Technology of China, Shanghai 201315, China*
[2]*Department of Physics and Zhejiang Institute of Modern Physics, Zhejiang University, Hangzhou, Zhejiang 310027, China*
[3]*Synergetic Innovation Center of Quantum Information and Quantum Physics, Hefei, Anhui 230026, China*
[4]*Laboratory of Quantum Engineering and Quantum Metrology, School of Physics and Astronomy, Sun Yat-Sen University (Zhuhai Campus), Zhuhai, Guangdong 519082, China*
[5]*Center for Measurements and Analyses, Zhejiang University of Technology, Hangzhou, Zhejiang 310014, China*
(Dated: October 29, 2019)

Here we present extra derivations and plots which may help with the understanding of the main text.

## I. EVOLUTION OF $1/k_Fa$ VERSUS $t$ AND ITS CONNECTION TO THE 2D LIMIT

To regularize the ultraviolet divergence in the integral of the gap equation (4) in the main text, we have introduced a scattering length $a$, via the Lippmann-Schwinger relation,

$$\frac{m}{4\pi a} = \frac{1}{U} + \sum_{\mathbf{k}} \frac{1}{2\epsilon_{\mathbf{k}}} \,. \tag{S1}$$

Due to the restricted momentum space in the lattice direction, this definition is similar to but different from its counterpart in isotropic 3D free space. In this definition, the anisotropy of the (effective) fermion mass was not considered. Needless to say, this scattering length parameter does not correspond to the actual scattering length when measured experimentally. Nonetheless, it can be regarded as an effective parameter for characterizing the interaction strength, just as in 3D continuum.

In the $t \to 0$ limit, where the system becomes 2D, this scattering length is rather different from the physical 2D $s$-wave scattering length, $a_{2D}$, which is given by

$$\epsilon_B = \frac{\hbar^2}{ma_{2D}^2} \,, \tag{S2}$$

where $\epsilon_B$ is the two-body binding energy. In the BEC regime, $\epsilon_B \approx -2\mu$. It should be noted, however, that $a_{2D}$ is always positive and diverges in the zero pairing strength limit, since an arbitrarily weak attractive interaction (including those of a finite range) is enough to form bound state in vacuum. Meanwhile, besides the ultraviolet divergence, infrared divergence also emerges in the momentum integral in the pair susceptibility $\chi(0)$ [See Eq. (S8) below] in exact 2D, as $t \to 0$. In exact 2D, the gap equation is regularized in a different way, via [1, 2]

$$\frac{1}{U} = -\sum_{\mathbf{k}} \frac{1}{\epsilon_B + 2\epsilon_{\mathbf{k}}} \,, \tag{S3}$$

which relates $1/U$ with $a_{2D}$. Since there is a logarithmic energy dependence in the low energy $s$-wave scattering phase shift, there is no easy way to define a single scattering length parameter which evolves continuously from 3D to 2D.

From Eq. (S1), it is clear that the infrared divergence at $t = 0$ leads to a logarithmic dependence of $1/a$ on $t$. Indeed, from Eq. (6) in the main text, we obtain in the BEC regime

$$\frac{1}{a} \approx \frac{1}{d} \ln \frac{|\mu|}{t} = -\frac{1}{d} \ln(2mta_{2D}^2) \,. \tag{S4}$$

We have checked Eq. (S4) numerically by solving our set of equations with fixed $\mu$ as a function of $t$. Shown in Fig. S1 is $1/k_Fa$ as a function of $t/E_F$ in a semi-log scale, calculated for $d = 2$ and $p = 0$ with $\mu/E_F = -10$ at low $T$ ($T_c$ to be precise). The perfect straight line fully verifies the logarithmic dependence given in Eq. (S4). Also shown is the analytical expression of Eq. (S4) (red dashed line), which overlays on top of the numerical solution except for the slight difference at large $t$, where the correction terms in Eq. (6) in the main text becomes quantitatively significant.

One should not be misled by Eq. (6) to think that the term $-te^{d/a}$ vanishes in the BEC limit as $t \to 0$. Instead, for a

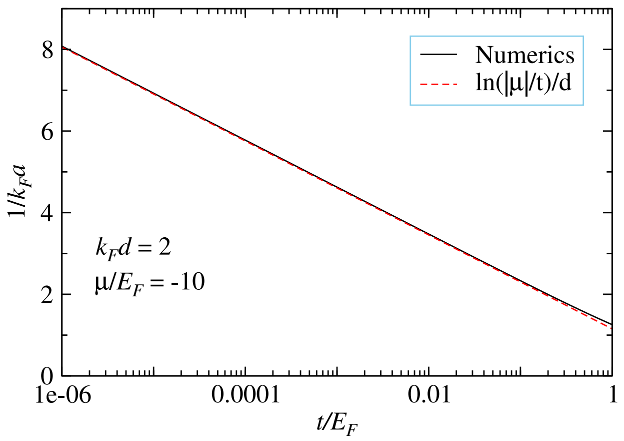


Figure S1. Behavior of $1/k_Fa$ as functions of $t/E_F$ in the BEC regime at fixed $\mu/E_F = -10$ for $k_Fd = 2$ and $p = 0$.

* Email: qchen@uchicago.edu
† Email: wangjibiao@gmail.com

given bind energy in the 2D limit, our $1/k_F a$ diverges logarithmically following Eq. (S4). On the other hand, for a fixed $1/k_F a$, $\mu$ approaches its noninteracting 2D value, ($\pi dn/m$ for $p=0$), as $t \to 0$, as we have verified numerically.

## II. EFFECTIVE SCATTERING LENGTH $a_{\text{eff}}$

The strong $t$ (and $d$) dependence of $a$ defined via Eq. (S1) suggests that the parameter $a$ is not comparable to the physical scattering length. Here we try to define an effective scattering length $a_{\text{eff}}$, which more or less reflects the physical scattering length.

Consider the long wave length limit of dispersion $\epsilon_{\mathbf{k}}$, and rescale $k_z$ such that $k'_z = \sqrt{2mtd}k_z$. Then for small $\mathbf{k}' \equiv (k_x, k_y, k'_z)$, we have

$$\epsilon_{\mathbf{k}'} = \frac{1}{2m}(\mathbf{k}_\parallel^2 + k_z'^2), \tag{S5}$$

which is isotropic in $\mathbf{k}'$. In this way, $\sum_{\mathbf{k}}$ becomes $\frac{1}{\sqrt{2mtd}}\sum_{\mathbf{k}'}$. Then the Lippmann-Schwinger equation becomes

$$\frac{m}{4\pi a_{\text{eff}}} \equiv \frac{m}{4\pi a}\sqrt{2mtd} = \frac{1}{U'} + \sum_{\mathbf{k}'} \frac{1}{2\epsilon_{\mathbf{k}'}}, \tag{S6}$$

where $U' = U/\sqrt{2mtd}$ is the rescaled interaction. Comparing this equation to the Lippmann-Schwinger equation in 3D free space, we expect the quantity $a_{\text{eff}} = a/\sqrt{2mtd}$ to be comparable to the physical scattering length.

## III. COEFFICIENTS OF THE INVERSE $T$ MATRIX EXPANSION IN THE BEC REGIME

In this section, we shall present explicit expressions for the equations and the coefficients associated with the Taylor expansion of the inverse $T$ matrix in the BEC regime.

The expressions for the coefficients of the inverse $T$ matrix expansion can be found in Ref. [3] for the balanced case and Ref. [4] for the imbalanced case. Here we just need to use the dispersion for a 1D optical lattice and assume $-\mu \gg T$ to further simplify the expressions. First, we list the expressions before taking the BEC approximation.

The pair susceptibility is

$$\chi(Q) = \frac{1}{2}\sum_K [G_{0\uparrow}(Q-K)G_\downarrow(K) + G_{0\downarrow}(Q-K)G_\uparrow(K)], \tag{S7}$$

with

$$\chi(0) = \sum_{\mathbf{k}} \frac{1-2\bar{f}(E_{\mathbf{k}})}{2E_{\mathbf{k}}}. \tag{S8}$$

Then the coefficient $a_0 = \frac{\partial}{\partial\Omega}\chi(\mathbf{q},\Omega)|_{\mathbf{q}=0,\Omega=0}$ is given by

$$\begin{aligned} a_0\Delta^2 &= \sum_{\mathbf{k}}\left[v_{\mathbf{k}}^2 + \frac{\xi_{\mathbf{k}}}{E_{\mathbf{k}}}\bar{f}(E_{\mathbf{k}}) - \bar{f}(\xi_{\mathbf{k}})\right] \\ &= \frac{n}{2} - \sum_{\mathbf{k}}\bar{f}(\xi_{\mathbf{k}}). \end{aligned} \tag{S9}$$

Not shown in Ref. [4], the expression for $a_1$ is

$$\begin{aligned} a_1 &= \frac{1}{2}\frac{\partial^2}{\partial\Omega^2}t^{-1}_{\mathbf{q},\Omega}\bigg|_{q=0,\Omega=0} \\ &= \frac{2}{\Delta^4}\sum_{\mathbf{k}} E_{\mathbf{k}}\left\{v_{\mathbf{k}}^4[1-2\bar{f}(E_{\mathbf{k}})] + \frac{\xi_{\mathbf{k}}}{E_{\mathbf{k}}}[\bar{f}(\xi_{\mathbf{k}}) - \bar{f}(E_{\mathbf{k}})]\right\}. \end{aligned} \tag{S10}$$

The coefficients in front of $\mathbf{q}^2$ are determined by

$$\begin{aligned} \frac{\partial^2\chi}{\partial\mathbf{q}^2} &= -\frac{1}{\Delta^2}\sum_{\mathbf{k}}\Bigg\{\left[v_{\mathbf{k}}^2 + \frac{\xi_{\mathbf{k}}}{E_{\mathbf{k}}}\bar{f}(E_{\mathbf{k}}) - \bar{f}(\xi_{\mathbf{k}})\right]\nabla^2\xi_{\mathbf{k}} \\ &\quad - \left[\frac{4E_{\mathbf{k}}}{\Delta^2}v_{\mathbf{k}}^4\big(1-2\bar{f}(E_{\mathbf{k}})\big) + 2\bar{f}'(\xi_{\mathbf{k}}) \right. \\ &\quad \left. + \frac{4\xi_{\mathbf{k}}}{\Delta^2}\big(\bar{f}(\xi_{\mathbf{k}}) - \bar{f}(E_{\mathbf{k}})\big)\right](\nabla\xi_{\mathbf{k}})^2\Bigg\} \\ &\equiv \frac{\partial^2\chi}{\partial\mathbf{q}_\parallel^2} \oplus \frac{\partial^2\chi}{\partial\mathbf{q}_z^2}, \end{aligned} \tag{S11}$$

where $\nabla^2\xi_{\mathbf{k}} = \frac{\partial^2\xi_{\mathbf{k}}}{\partial\mathbf{k}_\parallel^2} \oplus \frac{\partial^2\xi_{\mathbf{k}}}{\partial\mathbf{k}_z^2}$, and $(\nabla\xi_{\mathbf{k}})^2 = \left(\frac{\partial\xi_{\mathbf{k}}}{\partial\mathbf{k}_\parallel}\right)^2 \oplus \left(\frac{\partial\xi_{\mathbf{k}}}{\partial\mathbf{k}_z}\right)^2$. And

$$a_0(B_\parallel \oplus t_B d^2) = -\frac{1}{4}\frac{\partial^2\chi}{\partial\mathbf{q}_\parallel^2} \oplus \left(-\frac{1}{2}\right)\frac{\partial^2\chi}{\partial\mathbf{q}_z^2} \tag{S12}$$

Without showing all the lengthy but straightforward intermediate steps, here we will present the final result.

Defining dimensionless $I_1 \equiv J\sum_{\mathbf{k}} f(E_{\mathbf{k}}^\uparrow)$ and $I_2 \equiv J\sum_{\mathbf{k}} f(\xi_{\mathbf{k}}^\uparrow)$, with $J = \frac{\pi^2 d}{mt}$, then number difference equation in the BEC regime simplifies as

$$pn = I_1/J. \tag{S13}$$

The coefficient $a_0$ and the pair density $n_p$ are given by

$$n_p \equiv a_0\Delta^2 = \frac{n}{2} - \sum_{\mathbf{k}}\bar{f}(\xi_{\mathbf{k}}) = n_\downarrow - \frac{1}{2J}(I_2 - I_1). \tag{S14}$$

The coefficient $a_1$ is given by

$$a_1\Delta^2 = \frac{\pi}{8tJ^2 n_\downarrow}(I_2 - I_1) + \frac{n_\downarrow}{4|\mu|}\left(1 + \frac{\pi}{J^2 n_\downarrow^2}I_3\right), \tag{S15}$$

where the integral $I_3 = \frac{J}{2t}\sum_{\mathbf{k}}\epsilon_{\mathbf{k}}[f(\xi_{\mathbf{k}}^\uparrow) - f(E_{\mathbf{k}}^\uparrow)]$.

For the pair dispersion, we have

$$B_\parallel = \frac{1}{4m} + \frac{1}{8mJn_p}\left[(3I_2 + I_1) - \frac{\pi}{Jn_\downarrow}I_4\right], \tag{S16}$$

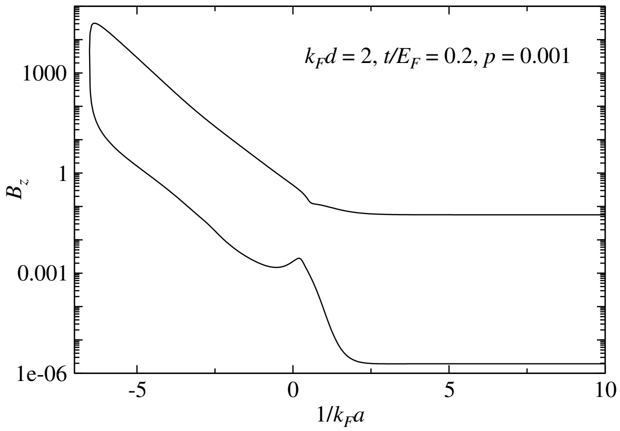


Figure S2. Behavior of $B_z$ as a function of $1/k_F a$ at fixed $k_F d = 2$, along the $T_c$ curve for $p = 0.001$ in Fig. 3 in the main paper.

where the first term is the $p = 0$ result, while the rest is contribution of population imbalance. The pair hopping integral $t_B$ is given by and

$$t_B = \frac{t^2}{n_p}\left\{\frac{1}{2tJ}\left(I_5 - I_6 + I_7 - \frac{\pi}{Jn_\downarrow}I_8\right) + \frac{n_\downarrow}{2|\mu|}\left(1 - \frac{8}{\pi}I_5 - \frac{4\pi}{J^2 n_\downarrow^2}I_9\right)\right\}, \tag{S17}$$

where $I_4 = \frac{J}{2mt}\sum_{\mathbf{k}}[f(\xi_{\mathbf{k}}^\uparrow) - f(E_{\mathbf{k}}^\uparrow)]k_\parallel^2$, $I_5 = J\sum_{\mathbf{k}} f(E_{\mathbf{k}}^\uparrow)c$, $I_6 = J\sum_{\mathbf{k}} f(\xi_{\mathbf{k}}^\uparrow)c$, $I_7 = -4tJ\sum_{\mathbf{k}} f'(\xi_{\mathbf{k}}^\uparrow)s^2$, $I_8 = J\sum_{\mathbf{k}}[f(\xi_{\mathbf{k}}^\uparrow) - f(E_{\mathbf{k}}^\uparrow)]s^2$, $I_9 = \frac{J}{2t}\sum_{\mathbf{k}}\epsilon_{\mathbf{k}}[f(\xi_{\mathbf{k}}^\uparrow) - f(E_{\mathbf{k}}^\uparrow)]s^2$, with $c \equiv \cos(k_z d)$, $s \equiv \sin(k_z d)$, and $n_p$ is to be replaced with Eq. (S14).

Note that all the integral $I$'s originate from the unpaired excessive majority fermions via the Fermi functions. When $p = 0$, all integral $I$'s vanish so that we recover $n_p = n_\downarrow = n/2$, $a_1\Delta^2 = -n/8\mu$, (which becomes exponentially small in the BEC limit), $B_\parallel = 1/4m$, and Eq. (S17) reduces to $t_B = t^2/2|\mu|$.

## IV. INTERMEDIATE TEMPERATURE SUPERFLUID

Figures 2 and 3 in the main text exhibit intermediate temperature superfluidity. This is in some way similar to the situation in homogeneous 3D Fermi gases with population imbalance [5]. We mention that intermediate temperature superfluid can already be found within the BCS mean-field theory [5]. Our calculations show that for given $1/k_F a$ and population imbalance $p$, as a function of $T$, the pair hopping matrix element $t_B$ in the lattice direction decreases with decreasing temperature from the upper to lower $T_c$, and would change sign soon below the lower $T_{c,L}$. As an example, we plot $B_z = t_B d^2$ along the $T_c$ curve for $p = 0.001$ in Fig. 3 of the main paper, as shown in Fig. S2. The upper and lower branches of $B_z$ correspond to the upper and lower $T_c$ branches, respectively. Clearly, there is a 3 to 5 orders of magnitude difference between these two branches. Below $T_{c,L}$, since $t_B$ would soon becomes negative, there would be phase separation, or FFLO-like pair density wave solutions.

## V. EFFECT OF $t$ ON $T_c$ AS A FUNCTION OF $1/k_F a$ FOR $k_F d = 2$ AND $p = 0.01$

In this section, we study the effect of $t$ on the behavior of $T_c$. Shown in Fig. S3 is $T_c$ as a function of $1/k_F a$ for fixed $k_F d = 2$ at $p = 0.01$, with a series of values of $t/E_F$, as labeled. The figure shows that for these parameters, the BEC superfluid phase exists only when $t/E_F \gtrsim 0.21$. For $t/E_F \lesssim 0.205$, The $T_c$ curve turns back somewhere on the BEC side of unitarity, and form a closed cycle. The enclosed superfluid phase shrinks as $t$ decreases further. As $t/E_F$ becomes very small, the $T_c$ curve moves downwards and gradually to the right, implying that a stronger pairing interaction is needed in order to form a superfluid. On the larger $t$ side, we notice that for $t/E_F \geq 0.25$, the lower $T_c$ branch bends down and vanishes at an intermediate pairing strength. In such a case, there exists a stable homogeneous polarized superfluid in the BEC regime at $T = 0$, similar to the case for the simple 3D continuum.

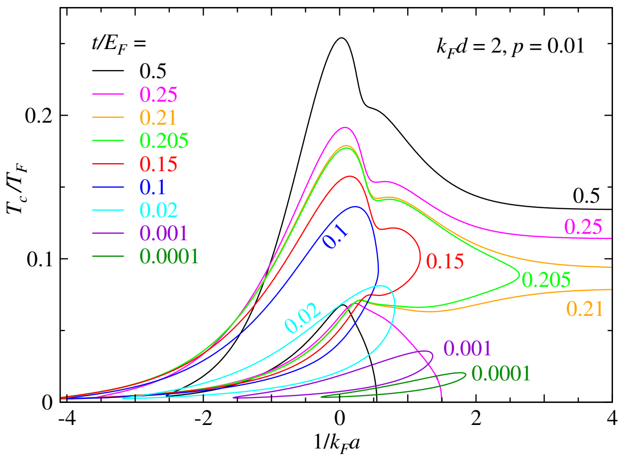


Figure S3. Behavior of $T_c$ as functions of $1/k_F a$ at fixed $k_F d = 2$ and $p = 0.01$, but for different values of $t/E_F$, as labeled.


[1] P. Bloom, Two-dimensional fermi gas, Phys. Rev. B **12**, 125 (1975).

[2] M. Randeria, J.-M. Duan, and L.-Y. Shieh, Superconductivity in a two-dimensional Fermi gas: Evolution from Cooper pairing to

Bose condensation, Phys. Rev. B **41**, 327 (1990).

[3] Q. J. Chen, *Generalization of BCS theory to short coherence length superconductors: A BCS-Bose-Einstein crossover scenario*, Ph.D. thesis, University of Chicago (2000), available as arXiv:1801.06266.

[4] Q. J. Chen, Y. He, C.-C. Chien, and K. Levin, Theory of superfluids with population imbalance: Finite-temperature and BCS-BEC crossover effects, Phys. Rev. B **75**, 014521 (2007).

[5] C.-C. Chien, Q. J. Chen, Y. He, and K. Levin, Intermediate temperature superfluidity in a Fermi gas with population imbalance, Phys. Rev. Lett. **97**, 090402 (2006).
